# Supplementary material for: Robust, Deep, and Reinforcement Learning for Management of Communication and Power Networks
Source: arXiv:2202.05395 source file (2022-02-08)
Supplement: Supplementary file 1 [file appendix.tex]

\chapter*{Appendix}\label{chap:app}

\subsection{Proof of Lemma \ref{lem:beta}}
\label{sec:lembeta}
%\begin{proof} 
%By homogeneity, it suffices to prove the case with $\|\bm{x}\|=1$, then $\bm{z}_0=\tilde{\bm{z}}_0$. 
By homogeneity of \eqref{eq:i1x}, it suffices to work with the case where $\|\bm{x}\|=1$.
It is easy to check that 
\begin{align}
\frac{1}{2}\left\|\bm{x}\bm{x}^\ccalT-\tilde{\bm{z}}_0\tilde{\bm{z}}_0^\ccalT\right\|_F
^2&=\frac{1}{2}\|\bm{x}\|^4+\frac{1}{2}\|\tilde{\bm{z}}_0\|^4-|\bm{x}^\ccalT\tilde{\bm{z}}_0|^2\nonumber\\
&=1-|\bm{x}^\ccalT\tilde{\bm{z}}_0|^2\nonumber\\
&=1-\cos^2\theta\label{eq:ineq1}
\end{align}
where $0\le \theta\le \pi/2$ is the angle between the spaces spanned by $\bm{x}$ and $\tilde{\bm{z}}_0$. Then one can write 
\begin{equation}
\label{eq:orth1}
\bm{x}=\cos\theta\,\tilde{\bm{z}}_0+\sin\theta\,\tilde{\bm{z}}_0^{\perp},
\end{equation}
where $\tilde{\bm{z}}_0^\perp\in \mathbb{R}^n$ is a unit vector that is orthogonal to $\tilde{\bm{z}}_0$ and has a nonnegative inner product with $\bm{x}$. 
Likewise,
\begin{equation}
\label{eq:orth2}
\bm{x}^{\perp}:=-\sin\theta\,\tilde{\bm{z}}_0+\cos\theta\,\tilde{\bm{z}}_0^{\perp},
\end{equation}
in which $\bm{x}^{\perp}\in\mathbb{R}^n$ is a unit vector orthogonal to $\bm{x}$. 

Since $\tilde{\bm{z}}_0$ is the solution to the maximum eigenvalue problem
\vspace{-.em}
\begin{align}\label{eq:maxeig1}
\tilde{\bm{z}}_0:=\arg\max_{\left\|\bm{z}\right\|=1}~&~\bm{z}^\ccalT\widebar{\bm{Y}}_0\bm{z}
\end{align}		
for $\widebar{\bm{Y}}_0:=\frac{1}{|\widebar{\mathcal{I}}_0|}\widebar{\bm{S}}^\ccalT_0\widebar{\bm{S}}_0$,
it is the leading eigenvector of $\widebar{\bm{Y}}_0$, i.e., $\widebar{\bm{Y}}_0\tilde{\bm{z}}_0=\lambda_{1}\tilde{\bm{z}}_0$, where $\lambda_1>0$ is the largest eigenvalue of $\widebar{\bm{Y}}_0$. 
Premultiplying \eqref{eq:orth1} and \eqref{eq:orth2} by $\widebar{\bm{S}}_0$ yields  
\begin{subequations}\label{eq:prem}
	\begin{align}
	\widebar{\bm{S}}_0	\bm{x}&=\cos\theta\,	\widebar{\bm{S}}_0\tilde{\bm{z}}_0+\sin\theta\,	\widebar{\bm{S}}_0\tilde{\bm{z}}_0^{\perp}\label{eq:prem1},\\
	\widebar{\bm{S}}_0	\bm{x}^{\perp}&=-\sin\theta\,	\widebar{\bm{S}}_0\tilde{\bm{z}}_0+\cos\theta\,	\widebar{\bm{S}}_0\tilde{\bm{z}}_0^{\perp}\label{eq:prem2}.
	%	\widebar{\bm{S}}_0\bm{x}&=\rho{\rm e}^{-j\phi(\tilde{\bm{z}}_0)}\widebar{\bm{S}}_0\tilde{\bm{z}}_0+\sqrt{1-\rho^2}\widebar{\bm{S}}_0\bm{v}\label{eq:prem1}\\
	%		\widebar{\bm{S}}_0\bm{u}&=-\sqrt{1-\rho^2}{\rm e}^{-j\phi(\tilde{\bm{z}}_0)}\widebar{\bm{S}}_0\tilde{\bm{z}}_0+\rho\widebar{\bm{S}}_0\bm{v},\label{eq:prem2}
	\end{align}	
	\end{subequations}
	Pythagoras' relationship now gives 
	\begin{subequations}\label{eq:prem}
		\begin{align}
		\big\|\widebar{\bm{S}}_0\bm{x}\big\|^2&=\cos^2\theta\big\|\widebar{\bm{S}}_0\tilde{\bm{z}}_0\big\|^2+\sin^2\theta\big\|\widebar{\bm{S}}_0\tilde{\bm{z}}_0^{\perp}\big\|^2\label{eq:prem11},\\
		\big\|\widebar{\bm{S}}_0\bm{x}^\perp\big\|^2&=\sin^2\theta\big\|\widebar{\bm{S}}_0\tilde{\bm{z}}_0\big\|^2+\cos^2\theta\big\|\widebar{\bm{S}}_0\tilde{\bm{z}}_0^{\perp}\big\|^2\label{eq:prem21},
		\end{align}	
		\end{subequations}
		where the cross-terms vanish because $\tilde{\bm{z}}_0^\ccalT\widebar{\bm{S}}_0^\ccalT\widebar{\bm{S}}_0\tilde{\bm{z}}_0^{\perp}=|\widebar{\mathcal{I}}_0|\tilde{\bm{z}}_0^\ccalT\widebar{\bm{Y}}_0\tilde{\bm{z}}_0^\perp=\lambda_1|\widebar{\mathcal{I}}_0|\tilde{\bm{z}}_0^\ccalT\tilde{\bm{z}}_0^{\perp}=0$ following from the definition of $\tilde{\bm{z}}^\perp_0$. 
		
		We next construct the following expression:
		\begin{align}
		&\sin^2\theta\big\|\widebar{\bm{S}}_0\bm{x}\big\|^2-\big\|\widebar{\bm{S}}_0\bm{x}^\perp\big\|^2\nonumber\\
		&=\sin^2\theta\Big(\cos^2\theta\big\|\widebar{\bm{S}}_0\tilde{\bm{z}}_0\big\|^2+\sin^2\theta\big\|\widebar{\bm{S}}_0\tilde{\bm{z}}_0^\perp\big\|^2\Big)\nonumber\\
		&\quad\,  -\Big(\sin^2\theta\big\|\widebar{\bm{S}}_0\tilde{\bm{z}}_0\big\|^2+\cos^2\theta\big\|\widebar{\bm{S}}_0\tilde{\bm{z}}_0^\perp \big\|^2\Big)\nonumber\\
		&=\sin^2\theta\Big(
		\cos^2\theta\big\|\widebar{\bm{S}}_0\tilde{\bm{z}}_0\big\|^2-\big\|\widebar{\bm{S}}_0\tilde{\bm{z}}_0\big\|^2+\sin^2\theta\big\|\widebar{\bm{S}}_0\tilde{\bm{z}}_0^\perp\big\|^2 \Big)-\nonumber\\
		&\quad\,
		\cos^2\theta\big\|\widebar{\bm{S}}_0\tilde{\bm{z}}_0^\perp \big\|^2\nonumber\\
		&=\sin^4\theta\Big(\big\|\widebar{\bm{S}}_0\tilde{\bm{z}}_0^\perp\big\|^2-\big\|\widebar{\bm{S}}_0\tilde{\bm{z}}_0\big\|^2\Big)-\cos^2\theta\big\|\widebar{\bm{S}}_0\tilde{\bm{z}}_0^\perp\big\|^2\label{eq:last11}\\
		&\le 0.\nonumber
		\end{align}
		Regarding the last inequality, since $\tilde{\bm{z}}_0$ maximizes the term $\tilde{\bm z}_0^\ccalT\widebar{\bm Y}_0\tilde{\bm z}_0=\frac{1}{|\widebar{\mathcal{I}}_0|}\tilde{\bm z}_0^\ccalT\widebar{\bm S}_0^\ccalT\widebar{\bm S}_0\tilde{\bm z}_0$ according to \eqref{eq:maxeig1}, then in \eqref{eq:last11} the first term $\|\widebar{\bm{S}}_0\tilde{\bm{z}}_0^\perp\|^2-\|\widebar{\bm{S}}_0\tilde{\bm{z}}_0\|^2\le 0$ holds for any unit vector $\tilde{\bm{z}}_0^\perp\in\mathbb{R}^n$. In addition, the second term $-\cos^2\theta\|\widebar{\bm{S}}_0\tilde{\bm{z}}_0^\perp\|^2\le 0$, thus yielding $\sin^2\theta\|\widebar{\bm{S}}_0\bm{x}\|^2-\|\widebar{\bm{S}}_0\bm{x}^\perp\|^2\le 0$. 
		%Upon rewriting $\|\widebar{\bm{S}}_0\bm{x}^\perp\|^2=\cos^2\theta\|\widebar{\bm{S}}_0\bm{x}^\perp\|^2+\sin^2\|\widebar{\bm{S}}_0\bm{x}^\perp\|^2 $, one arrives at
		For any nonzero $\bm{x}\in\mathbb{R}^n$, 
		it holds that
		\begin{equation}
		\sin^2\theta=1-\cos^2\theta \le \frac{\big\|\widebar{\bm{S}}_0\bm{x}^\perp\big\|^2}{\big\|\widebar{\bm{S}}_0\bm{x}\big\|^2}.
		\end{equation}
		Upon letting $\bm{u}=\bm{x}^\perp$, the last inequality taken together with \eqref{eq:ineq1} concludes the proof of \eqref{eq:mse}.
		%\end{proof}

		\subsection{Proof of Lemma \ref{lem:up}}\label{sec:proofup}
		
		Assume $\|\bm{x}\|=1$.
		Let $\bm{s}\in\mathbb{R}^n$ be sampled uniformly at random on the unit sphere, which has zero mean and covariance matrix $\bm{I}_n/n$. 
		%By the rotational invariance of the uniformly spherical distribution, 
		Let also $\bm{U}\in\mathbb{R}^{n\times n}$ be a unitary matrix such that $\bm{U}\bm{x}=\bm{e}_1$, where $\bm{e}_1$ is the first canonical vector in $\mathbb{R}^n$. It is then easy to verify that the following holds for any fixed threshold $0<\tau<1$ \cite{duchi2017}:
		\allowdisplaybreaks
		\begin{align}
		\label{eqq:exp}
		&\mathbb{E}[\bm{s}\bm{s}^\ccalT|(\bm{s}^\ccalT\bm{x})^2>\tau]\nonumber\\
		&=\bm{U}\mathbb{E}[\bm{U}^\ccalT\bm{s}\bm{s}^\ccalT\bm{U}|(\bm{s}^\ccalT\bm{U}\bm{U}^\ccalT\bm{x})^2>\tau]\bm{U}^\ccalT\nonumber\\
		&\buildrel(i)\over = \bm{U}\mathbb{E}[\tilde{\bm{s}}\tilde{\bm{s}}^\ccalT|(\tilde{\bm{s}}^\ccalT\bm{e}_1)^2>\tau]\bm{U}^\ccalT\nonumber\\
		& = \bm{U}\mathbb{E}[\tilde{\bm{s}}\tilde{\bm{s}}^\ccalT|\tilde{s}_1^2>\tau]\bm{U}^\ccalT\nonumber\\
		& = \bm{U}\left[\begin{array}{ll} \mathbb{E}[\tilde{s}_1^2|\tilde{s}_1^2>\tau] &\mathbb{E}[\tilde{s}_1\tilde{\bm{s}}_{\backslash1}^\ccalT|\tilde{s}_1^2>\tau]\\
		\mathbb{E}[\tilde{s}_1\tilde{\bm{s}}_{\backslash1}|\tilde{s}_1^2>\tau]&\mathbb{E}[\tilde{\bm{s}}_{\backslash1}\tilde{\bm{s}}_{\backslash1}^\ccalT|\tilde{s}_1^2>\tau]
		\end{array}\right]\bm{U}^\ccalT\nonumber\\
		&\buildrel(ii)\over = \bm{U}\left[\begin{array}{ll} \mathbb{E}[\tilde{s}_1^2|\tilde{s}_1^2>\tau] &\bm{0}^\ccalT\\
		\bm{0}&\mathbb{E}[\tilde{\bm{s}}_{\backslash1}\tilde{\bm{s}}_{\backslash1}^\ccalT|\tilde{s}_1^2>\tau]
		\end{array}\right]\bm{U}^\ccalT\nonumber\\
		&\buildrel(iii)\over = \mathbb{E}[\tilde{s}_2^2|\tilde{s}_1^2>\tau]
		\bm{I}_n+\big( \mathbb{E}[\tilde{s}_1^2|\tilde{s}_1^2>\tau]- \mathbb{E}[\tilde{s}_2^2|\tilde{s}_1^2>\tau]\big)\bm{x}\bm{x}^\ccalT\nonumber\\
		&\buildrel\triangle\over =C_1\bm{I}_n+C_2\bm{x}\bm{x}^\ccalT
		\end{align}
		with the constants $C_1:=\mathbb{E}[\tilde{s}_2^2|\tilde{s}_1^2>\tau]<\frac{1-\tau}{n-1}$, $C_2:= \mathbb{E}[\tilde{s}_1^2|\tilde{s}_1^2>\tau]- C_1>0$, and  $\bm{s}_{\backslash 1}\in\mathbb{R}^{n-1}$  denoting the subvector of $\bm{s}\in\mathbb{R}^n$ after removing the first entry from $\bm{s}$. Here, the result $(i)$ follows upon defining $\tilde{\bm{s}}:=\bm{U}^\ccalT\bm{s}$, which obeys the uniformly spherical distribution too using the rotational invariance. The equality $(ii)$ is due to the zero-mean and symmetrical properties of the uniformly spherical distribution. Finally, to derive $(iii)$, we have used the fact $\bm{x}=\bm{U}\bm{e}_1=\bm{u}_1$, the first column of $\bm{U}$, which arises from $\bm{U}^\ccalT\bm{x}=\bm{e}_1$ and $\bm{U}\bm{U}^\ccalT=\bm{I}_n$.
		
		By the argument above, assume without loss of generality that $\bm{x}=\bm{e}_1$. Consider now the truncated vector $\bm{s}_{\backslash 1}|(\bm{s}^\ccalT\bm{x})^2>\tau$, or equivalently, $\bm{s}_{\backslash 1}|s_1^2>\tau$. 
		It is then clear that $\bm{s}_{\backslash 1}|s_1^2>\tau$ is bounded, and thus subgaussian; furthermore, the next hold
		\begin{subequations}
			\begin{align}
			\mathbb{E}[\bm{s}_{\backslash 1}|s_1^2>\tau]&=\bm{0}\\
			\mathbb{E}\big[\big(\bm{s}_{\backslash 1}|s_1^2>\tau\big) \big(\bm{s}_{\backslash 1}|s_1^2>\tau\big)^\ccalT\big]&=C_1\bm{I}_{n-1}\label{eqq:cov}
			\end{align}
			\end{subequations}
			where \eqref{eqq:cov} is obtained as a submatrix of the first term in \eqref{eqq:exp} since the second term $C_2\bm{e}_1\bm{e}_1^\ccalT$ is removed.

			Considering a unit vector $\bm{x}^\perp$ such that 
			$\bm{x}^\ccalT\bm{x}^\perp=\bm{e}_1^\ccalT\bm{x}^\perp=0$, there exists a unit vector $\bm{d}\in\mathbb{R}^{n-1}$ such that $\bm{x}^\perp=\left[0~\bm{d}^\ccalT\right]^\ccalT$. Thus, it holds that  
			\begin{equation}\label{eq:su}
			\big\|\widebar{\bm{S}}_0\bm{x}^\perp\big\|^2
			=\Big\|\widebar{\bm{S}}_0\big[0~\bm{d}^\ccalT\big]^\ccalT\Big\|^2=\big\|\widebar{\bm{S}}_{0, \backslash 1}\bm{d}\big\|^2
			\end{equation}
			where $\widebar{\bm{S}}_{0, \backslash 1}\in\mathbb{R}^{|\widebar{\mathcal{I}}_0|\times (n-1)}$ is obtained through deleting the first column in $\widebar{\bm{S}}_0$, which is denoted by $\widebar{\bm{S}}_{0,1}$; that is, $\widebar{\bm{S}}_0=\big[\widebar{\bm{S}}_{0,1}~\widebar{\bm{S}}_{0, \backslash 1}\big]$.
			%Letting $\bm{F}:=\big[\bm{f}_1~\cdots~\bm{f}_{|\widebar{\mathcal{I}}_0|} \big]^\ccalT$, one can readily write $\bm{s}_i=\big[s_{i,1}~\bm{f}_i^\ccalT\big]^\ccalT$,~$\forall i\in[|\widebar{\mathcal{I}}_0|]:=\{1,\ldots,|\widebar{\mathcal{I}}_0|\}$.
			
			The rows of $\widebar{\bm{S}}_{0, \backslash 1}$ may therefore be viewed as independent realizations of the conditional random vector $\bm{s}_{\backslash 1}^\ccalT|s_1^2>\tau$, with the threshold $\tau$ being the  $|\widebar{\mathcal{I}}_0|$-largest value in $\{y_i/\|\bm{a}_i\|^2\}_{i=1}^m$. 
			Standard concentration inequalities on the sum of random positive semi-definite matrices composed of independent non-isotropic subgaussian rows~\cite[Remark 5.40]{chap2010vershynin} confirm that 
			\begin{equation}\label{eq:iso}
			\left\|\tfrac{1}{|\widebar{\mathcal{I}}_0|}\widebar{\bm{S}}_{0, \backslash 1}^\ccalT\widebar{\bm{S}}_{0, \backslash 1}-C_1\bm{I}_{n-1}\right\|\le \sigma C_1 \le  \frac{(1-\tau)\sigma}{n-1}
			\end{equation}
			holds with probability at least $1-2{\rm e}^{-c_K n}$ as long as $|\widebar{\mathcal{I}}_0|/n$ is sufficiently large, where
			$\sigma$ is a numerical constant that can take arbitrarily small values, and $c_K>0$ is a universal constant. 
			Without loss of generality, let us work with $\sigma:=0.005$ in~\eqref{eq:iso}.
			Then for any unit vector $\bm{d}\in\mathbb{R}^{n-1}$, the following inequality holds with probability at least $1-2{\rm e}^{-c_K n}$:
			%On the other hand, for any unit vector $\bm{x}^\perp\in\mathbb{R}^{n}$, define the new random variable $\nu:=(\bm{s}^\ccalT\bm{x}^\perp)^2|(\bm{s}^\ccalT\bm{x})^2>\tau$, whose mean is $\mathbb{E}[\nu]=\mathbb{E}[(\bm{s}^\ccalT\bm{x}^\perp)^2|(\bm{s}^\ccalT\bm{x})^2>c]=C_1(\bm{x}^\perp)^\ccalT\bm{x}^\perp=C_1$ using \eqref{eqd:exp}. That is, $\tfrac{1}{|\widebar{\mathcal{I}}_0|}
			%(\bm{x}^\perp)^\ccalT\bm{S}^\ccalT\bm{S}\bm{x}^\perp$ is the average of $|\widebar{\mathcal{I}}_0|$ independent subgaussian random variables with subgaussian norm $cC_1$  By means of Hoeffding-type inequality \cite[Proposition 5.10]{chap2010vershynin},
			% the following inequality holds with probability at least $1-2{\rm e}^{-c_K n}$:
			\begin{equation}
			\left|\tfrac{1}{|\widebar{\mathcal{I}}_0|}\bm{d}^\ccalT\widebar{\bm{S}}_{0,\backslash 1}^\ccalT\widebar{\bm{S}}_{0,\backslash 1}\bm{d}-C_1\right|\le  \frac{0.01}{n}
			\end{equation}
			for $n\ge 3$.
			Therefore, one readily concludes that
			\begin{equation}\label{eq:up}
			\big\|\widebar{\bm{S}}_0\bm{x}^\perp\big\|^2=\left|(\bm{x}^\perp)^\ccalT\bm{S}^\ccalT\bm{S}\bm{x}^\perp\right|\le {1.01|\widebar{\mathcal{I}}_0|}\big/{n}
			%\left(1+\maximize\left(\delta,\delta^2\right)\right).
			%\left|\frac{1}{|\widebar{\mathcal{I}}_0|}\bm{d}^\ccalT\bm{H}^\ccalT\bm{H}\bm{d}-\frac{1}{n}\bm{d}^\ccalT\bm{d} \right|\le \frac{1}{n} \maximize(\delta,\delta^2)\bm{d}^\ccalT\bm{d}
			\end{equation}
			holds with probability at least $1-2{\rm e}^{-c_K n}$, provided that $|\widebar{\mathcal{I}}_0|\big/n$ exceeds some constant. Note that $c_K$ depends on the maximum subgaussian norm of rows of $\bm{S}$, and we assume without loss of generality $c_K\ge 1/2$. Hence, $\|\widebar{\bm{S}}_0\bm{u}\|^2$ in~\eqref{eq:mse}
			is upper bounded simply by letting $\bm{u}=\bm{x}^\perp$ in~\eqref{eq:up}.

			\subsection{Proof of Lemma \ref{lem:low}}\label{sec:prooflow}

			%Albeit the nominator term $\big\|\widebar{\bm{S}}_0\bm{x}^\perp\big\|^2$ in~\eqref{eq:mse} is upper bounded, another challenge consists in pursuing 
			We next pursue a meaningful lower bound for $\|\widebar{\bm{S}}_0\bm{x}\|^2$ in~\eqref{eq:low0}. When $\bm{x}=\bm{e}_1$, one has $\|\widebar{\bm{S}}_0\bm{x}\|^2=\|\widebar{\bm{S}}_0\bm{e}_1\|^2=\sum_{i=1}^{|\widebar{\mathcal{I}}_0|}\bar{s}_{i,1}^2$, where $\{\bar{s}_{i,1}\}_{i=1}^{|\widebar{\mathcal{I}}_0|}$ are entries of the first column of $\widebar{\bm{S}}_0$.
			It is further worth mentioning that all squared entries of any spherical random vector obey the \emph{Beta} distribution with parameters $\alpha=\frac{1}{2}$, and $\beta=\frac{n-1}{2}$, i.e., $\bar{s}^2_{i,j}\sim {\rm Beta}\!\left(\frac{1}{2},\,\frac{n-1}{2}\right)$ for all $i,\,j$,~\cite[Lemma 2]{1981ecd}. Although they have closed-form probability density functions (pdfs) that may facilitate deriving a lower bound, 
			we take another route detailed as follows. A simple yet useful inequality is established first.
			
			\begin{lemma}
				\label{lem:max}
				Given $m$ fractions obeying $1>\frac{p_1}{q_1}\ge \frac{p_2}{q_2}\ge \cdots\ge\frac{p_m}{q_m}>0$, in which $p_i,\,q_i>0$, $\forall i\in[m]$, the following holds for all $1\le k\le m$
				\begin{equation}\label{eq:ineq}
				\sum_{i=1}^{k}\frac{p_{i}}{q_{i}}\ge \sum_{i=1}^k\frac{p_{[i]}}{q_{[1]}}
				\end{equation} 
				where $p_{[i]}$ denotes the $i$-th largest one among $\{p_i\}_{i=1}^m$, and hence, $q_{[1]}$ is the maximum in $\{q_i\}_{i=1}^m$.  
				\end{lemma} 
				
				\begin{proof}
					%	We prove the lemma by mathematical induction. For $k=1$, if $p_1=p_{[1]}$, since $q_1\le q_{[1]}$, the result $\frac{p_1}{q_1}\ge \frac{p_{[1]}}{q_{[1]}}$ holds. 
					%If $p_1<p_{[1]}$, letting $j_i\in[m]$ be the index such that $p_{j_{i}}=p_{[i]}$, then $\frac{p_1}{q_1}\ge\frac{p_{[1]}}{q_{j_1}}\ge \frac{p_{[1]}}{q_{[1]}}$ due to $q_{[1]}\ge q_{j_{1}}$. Hence, the result holds for $k=1$.
					%
					%Suppose the inequality in \eqref{eq:ineq} holds for $k=n<m$; that is, 
					%$		\sum_{i=1}^{n}\frac{p_{i}}{q_{i}}\ge \sum_{i=1}^n\frac{p_{[i]}}{q_{[1]}}
					%$.	 When $k=n+1$, $\sum_{i=1}^{n+1}\frac{p_{i}}{q_{i}}\ge \sum_{i=1}^n\frac{p_{[i]}}{q_{[1]}}+\frac{p_{n+1}}{q_{n+1}}$. To prove  \eqref{eq:ineq}, it suffices to prove $\frac{p_{n+1}}{q_{n+1}}\ge \frac{p_{[n+1]}}{q_{[1]}}$. If $p_{n+1}\ge p_{[n+1]}$, considering $q_{n+1}\le q_{[1]}$, so $\frac{p_{n+1}}{q_{n+1}}\ge \frac{p_{[n+1]}}{q_{[1]}}$ holds. If, on the other hand, $p_{n+1}<p_{[n+1]}$, since $\frac{p_{n+1}}{q_{n+1}}\ge \frac{p_{[n+1]}}{q_{j_{n+1}}}$, then the result follows. 
					For any $k\in[m]$, according to the definition of $q_{[i]}$, it holds that $p_{[1]}\ge p_{[2]}\ge \cdots\ge p_{[k]}$, so $\frac{p_{[1]}}{q_{[1]}}\ge \frac{p_{[2]}}{q_{[1]}}\ge \cdots\ge \frac{p_{[k]}}{q_{[1]}}$. Considering $q_{[1]}\ge q_{i}$, $\forall i\in [m]$, and letting $j_i\in[m]$ be the index such that $p_{j_{i}}=p_{[i]}$,  
					then $\frac{p_{j_i}}{q_{j_i}}=\frac{p_{[i]}}{q_{j_i}}\ge \frac{p_{[i]}}{q_{[1]}}$ holds for any $i\in[k]$. Therefore, 
					$\sum_{i=1}^k\frac{p_{j_i}}{q_{j_i}}=
					\sum_{i=1}^k\frac{p_{[i]}}{q_{j_i}}\ge \sum_{i=1}^k\frac{p_{[i]}}{q_{[1]}}$. Note that $\left\{\frac{p_{[i]}}{q_{j_i}}\right\}_{i=1}^k$ comprise a subset of terms in $\left\{\frac{p_i}{q_i}\right\}_{i=1}^m$. On the other hand, according to our assumption, $\sum_{i=1}^k\frac{p_i}{q_i}$ is the largest among all sums of $k$ summands; hence, $\sum_{i=1}^k\frac{p_i}{q_i}\ge \sum_{i=1}^k\frac{p_{[i]}}{q_{j_i}}$ yields
					$\sum_{i=1}^k\frac{p_i}{q_i}\ge \sum_{i=1}^k\frac{p_{[i]}}{q_{[1]}}$ concluding the proof.   
					\end{proof}

							Without loss of generality and for simplicity of exposition, let us assume that indices of $\bm{a}_i$'s have been re-ordered such that
							\begin{equation}\label{eq:allai}
							\frac{a_{1,1}^2}{\left\|\bm{a}_{1}\right\|^2}\ge \frac{a_{2,1}^2}{\left\|\bm{a}_{2}\right\|^2}\ge \cdots \ge \frac{a_{m,1}^2}{\left\|\bm{a}_{m}\right\|^2},
							\end{equation}
							where $a_{i,1}$ denotes the first element of $\bm{a}_i$.
							Therefore, writing
							$	\|\widebar{\bm{S}}_0\bm{e}_1\|^2=\sum_{i=1}^{|\widebar{\mathcal{I}}_0|}a_{i,1}^2/\|\bm{a}_{i}\|^2
							$, the next task  
							amounts to finding the sum of the $|\widebar{\mathcal{I}}_0|$ largest out of all $m$ entities in \eqref{eq:allai}.
							Applying the result \eqref{eq:ineq} in Lemma \ref{lem:max} gives
							\begin{equation}\label{eq:mid}
							%\left\|\widebar{\bm{S}}_0\bm{e}_1\right\|^2=
							\sum_{i=1}^{|\widebar{\mathcal{I}}_0|}\frac{a_{i,1}^2}{\left\|\bm{a}_{i}\right\|^2}\ge \sum_{i=1}^{|\widebar{\mathcal{I}}_0|}\frac{a_{[i],1}^2}{\max_{i\in[m]}\left\|\bm{a}_i\right\|^2},
							\end{equation}  
							in which $a_{[i],1}^2$ stands for the $i$-th largest entity in $\left\{a^2_{i,1}\right\}_{i=1}^m$. 
							
							Observe that for i.i.d. random vectors $\bm{a}_i\sim\mathcal{N}\big(\bm{0},\bm{I}_n\big)$, the property $\mathbb{P}(\left\|\bm{a}_i\right\|^2\ge 2.3n)\le {\rm e}^{-n/2}$ holds for large enough $n$ (e.g., $n\ge 20$),
							which can be understood upon substituting $\xi:=n/2$ into the following standard result~\cite[Lemma 1]{chisquaretail}
							\begin{equation}
							\mathbb{P}\left(\left\|\bm{a}_i\right\|^2-n\ge 2\sqrt{\xi}+2\xi \right)\le {\rm e}^{-\xi}.
							\end{equation}  
							In addition, one readily concludes that  
							$\mathbb{P}\left(\max_{i\in[m]}\left\|\bm{a}_i\right\|\le \sqrt{2.3n}\right)\ge 1-m{\rm e}^{-n/2}$. We will henceforth build our subsequent proofs on this event without stating this explicitly each time encountering it. Therefore, \eqref{eq:mid} can be lower bounded by
							\begin{align}
							\big\|\widebar{\bm{S}}\bm{x}\big\|^2=
							\sum_{i=1}^{|\widebar{\mathcal{I}}_0|}\frac{a_{i,1}^2}{\left\|\bm{a}_{i}\right\|^2}
							&\ge \sum_{i=1}^{|\widebar{\mathcal{I}}_0|}\frac{a_{[i],1}^2}{\max_{i\in[m]}\left\|\bm{a}_i\right\|^2}\nonumber\\
							&\ge \frac{1}{2.3n}\sum_{i=1}^{|\widebar{\mathcal{I}}_0|}{\left|a_{[i],1}\right|^2}\label{eq:down}
							\end{align}
							which holds with probability at least $1-m{\rm e}^{-n/2}$. 
							The task left for bounding $\|\widebar{\bm{S}}\bm{x}\|^2$
							is to derive a meaningful lower bound for $\sum_{i=1}^{|\widebar{\mathcal{I}}_0|}{a_{[i],1}^2}$. 
							%\textcolor{red}{
							Roughly speaking, because the ratio ${|\widebar{\mathcal{I}}_0|}/{m}$ is small, e.g., ${|\widebar{\mathcal{I}}_0|}/{m}\le 1/5$, a trivial result consists of bounding $(1/|\widebar{\mathcal{I}}_0|) \sum_{i=1}^{|\widebar{\mathcal{I}}_0|}{a_{[i],1}^2}$ by its sample average 
							$(1/m) \sum_{i=1}^{m}{a_{[i],1}^2}$.
							The latter can be bounded using its ensemble mean, i.e., $\mathbb{E}[a_{i,1}^2]=1$, $\forall i\in[\widebar{\mathcal{I}}_0]$, to yield $(1/m) \sum_{i=1}^{m}{a_{[i],1}^2}\ge (1-\epsilon)\mathbb{E}[a_{i,1}^2]=1-\epsilon$, which holds with high probability for some numerical constant $\epsilon>0$~\cite[Lemma 3.1]{phaselift}. Therefore, one has a candidate lower bound $\sum_{i=1}^{|\widebar{\mathcal{I}}_0|}{a_{[i],1}^2}\ge (1-\epsilon) |\widebar{\mathcal{I}}_0|$. 
							Nonetheless, this lower bound is in general too loose, and it contributes to a relatively large upper bound on the wanted term in \eqref{eq:mse}.

							To obtain an alternative bound, let us examine first the typical size of the maximum in $\left\{a_{i,1}^2\right\}_{i=1}^m$. Observe obviously that the modulus $\left|a_{i,1}\right|$ follows the half-normal distribution having the pdf $p(r)=\sqrt{{2}/{\pi}}\cdot {\rm e}^{-{r^2}/{2}}$, $r> 0$, and it is easy to verify that 
							\begin{equation}\label{eq:halfnormalmean}
							\mathbb{E}[|a_{i,1}|]=\sqrt{2/\pi}.
							\end{equation}
							Then integrating the pdf from $0$ to $+\infty$ yields the corresponding accumulative distribution function~(cdf) expressible in terms of the error function 
							$	\mathbb{P}\left(\left|a_{i,1}\right|>\xi\right)=1-{\rm erf}\left({\xi}/{2}\right)$, i.e., ${\rm erf}\left(\xi\right):={2}/{\sqrt{\pi}}\cdot \int_{0}^\xi{\rm e}^{-r^2}{\rm d}r$. Appealing to a lower bound on the complimentary error function ${\rm erfc}\left(\xi\right):=1-{\rm erf}\left(\xi\right)$ from~\cite[Theorem 2]{erf2011}, one establishes that 
							$\mathbb{P}\left(\left|a_{i,1}\right|>\xi\right)=1-{\rm erf}\left({\xi}/{2}\right)\ge (3/5){\rm e}^{-{\xi^2}/{2}}
							$. % beta=2, alpha=1/2<0.65
							Additionally, direct application of probability theory and Taylor expansion confirms that
							\begin{align}\label{eq:highp}
							\mathbb{P}\big(\max_{i\in[m]}\left|a_{i,1}\right|\ge \xi\big)&=1-\left[\mathbb{P}\left(\left|a_{i,1}\right|\le \xi\right)\right]^m\nonumber\\
							&\ge 1-\left(1-0.6{\rm e}^{-{\xi^2}/{2}}\right)^m\nonumber\\
							&\ge 1-{\rm e}^{-{0.6m}{\rm e}^{-\xi^2/2}}.
							%&\ge \frac{m}{2}{\rm e}^{-\frac{\xi^2}{\sqrt{2}}}-\frac{m^2}{8}{\rm e}^{-\sqrt{2}\xi^2}.	
							\end{align}
							Choosing now $\xi:=\sqrt{2\log n}$ leads to 
							\begin{equation}
							\mathbb{P}\big(\max_{i\in[m]}\left|a_{i,1}\right|\ge \sqrt{2\log n}\big)\ge 1-{\rm e}^{-0.6m/n}\ge 1-o(1)
							\label{eq:logn}	
							\end{equation}
							which holds with the proviso that $m/n$ is large enough, and the symbol $o(1)$ represents a small constant probability. 
							Thus, provided that $m/n$ exceeds some large constant, the event $\max_{i\in [m]} a_{i,1}^2\ge 2\log n$ occurs with high probability. Hence, one may expect a tighter lower bound than $(1-\epsilon_0)|\widebar{\mathcal{I}}_0|$, which is on the same order of $m$ under the assumption that $|\widebar{\mathcal{I}}_0|/m$ is about a constant.
							% and derived a straightforward deviation bound result of $\sum_{i=1}^{|\widebar{\mathcal{I}}_0|}{a_{[i],1}^2}$ from its mean.  
							
							% \asymp
							% \gtrsim
							% \lesssim
							
							Although $a_{i,1}^2$ obeys the \emph{Chi-square} distribution with $k=1$ degrees of freedom, its cdf is rather complicated and does not admit a nice closed-form expression. A small trick is hence taken in the sequel. Assume without loss of generality that both $m$ and $|\widebar{\mathcal{I}}_0|$ are even. Grouping two consecutive $a_{[i],1}^2$'s together, introduce a new variable $\vartheta{[i]}:=a_{[2k-1],1}^2+a_{[2k],1}^2$, $\forall k\in[{m}/{2}]$, 
							%whence $m$ is assumed even without loss of generality, 
							hence yielding a sequence of ordered numbers, i.e., $\vartheta_{[1]}\ge \vartheta_{[2]}\ge \cdots \ge \vartheta_{[m/2]}>0
							$. Then, one can equivalently write the wanted sum as 
							\begin{equation}
							\sum_{i=1}^{|\widebar{\mathcal{I}}_0|}a_{[i],1}^2=\sum_{i=1}^{|\widebar{\mathcal{I}}_0|/2}\vartheta_{[i]}. 
							\label{eq:rsum}	
							\end{equation}

							On the other hand, for i.i.d. standard normal random variables $\left\{a_{i,1}\right\}_{i=1}^m$, let us consider grouping randomly two of them and denote the corresponding sum of their squares by $\chi_{k}:=a_{k_i,1}^2+a_{k_j,1}^2$, where $k_i\ne k_j\in[m]$, and $k\in[m/2]$. It is self-evident that the $\chi_k$'s are identically distributed obeying the \emph{Chi-square} distribution with $k=2$ degrees of freedom, having the pdf 
							\begin{equation}\label{eq:chipdf}
							p\left(r\right)=\frac{1}{2}{\rm e}^{-\frac{r}{2}},\quad r\ge 0,
							\end{equation}
							and the following complementary cdf (ccdf)
							\begin{equation}\label{eq:chiccdf}
							\mathbb{P}\!\left(\chi_k\ge \xi\right):=\int_{\xi}^{\infty}\frac{1}{2}{\rm e}^{-\frac{r}{2}}{\rm d}r={\rm e}^{-\frac{\xi}{2}},\quad\forall \xi\ge 0.
							\end{equation}
							Ordering all $\chi_k$'s, summing the $|\widebar{\mathcal{I}}_0|/2$ largest ones, and comparing the resultant sum with the one in~\eqref{eq:rsum} confirms that 
							\begin{equation}\label{eq:relation}
							\sum_{i=1}^{|\widebar{\mathcal{I}}_0|/2}\chi_{[i]}\le \sum_{i=1}^{|\widebar{\mathcal{I}}_0|/2}\vartheta_{[i]}=\sum_{i=1}^{|\widebar{\mathcal{I}}_0|}a_{[i],1}^2,\quad \forall |\widebar{\mathcal{I}}_0|\in [m].
							\end{equation} 
							
							Upon setting $\mathbb{P}\!\left(\chi_k\ge \xi\right)={|\widebar{\mathcal{I}}_0|}/{m}$, one obtains an estimate of $\chi_{|\widebar{\mathcal{I}}_0|/2}$, the $(|\widebar{\mathcal{I}}_0|/2)$-th largest value in $\left\{\chi_k\right\}_{k=1}^{m/2}$ as follows
							\begin{equation}
							\hat{\chi}_{|\widebar{\mathcal{I}}_0|/2}:=2\log\big(m\big/|\widebar{\mathcal{I}}_0|\big).
							\end{equation}
							Furthermore, applying the Hoeffding-type inequality~\cite[Proposition 5.10]{chap2010vershynin} and leveraging the convexity of the ccdf in \eqref{eq:chiccdf}, one readily establishes that
							\begin{equation}\label{eq:hoeffding1}
							\mathbb{P}\!\left(\hat{\chi}_{|\widebar{\mathcal{I}}_0|/2}-\chi_{|\widebar{\mathcal{I}}_0|/2}>\xi \right)\le {\rm e}^{-\frac{1}{4}m\xi^2{\rm e}^{-\xi}(|\widebar{\mathcal{I}}_0|/m)^2},\quad\forall \xi>0.
							\end{equation}
							%\begin{equation}\label{eq:hoeffding1}
							%\mathbb{P}\!\left(\hat{\chi}_{|\widebar{\mathcal{I}}_0|/2}-\chi_{|\widebar{\mathcal{I}}_0|/2}>\xi \right)\le {\rm e}^{-\frac{1}{4}\xi^2{\rm e}^{-\xi}|\widebar{\mathcal{I}}_0|^2/m},~\forall \xi>0
							%\end{equation}
							%for which more details can be found in~\cite[Proposition A.3.]{2015chen1}. 
							Taking without loss of generality $\xi:=0.05 \hat{\chi}_{|\widebar{\mathcal{I}}_0|/2}=0.1\log\big(m\big/|\widebar{\mathcal{I}}_0|\big)$ gives
							\begin{equation}\label{eq:hoeffding}
							\mathbb{P}\!\left(\chi_{|\widebar{\mathcal{I}}_0|/2}<0.95\hat{\chi}_{|\widebar{\mathcal{I}}_0|/2} \right)\le {\rm e}^{-c_{0}m
								}
								\end{equation}
								for some universal constants $c_{0},\, c_{\chi}>0$, and sufficiently large $n$ such that ${|\widebar{\mathcal{I}}_0|}/{m}\gtrsim c_{\chi}>0$. %c_{\chi}
								%Setting $\xi:=\epsilon \hat{\chi}_{|\widebar{\mathcal{I}}_0|/2}=2\epsilon\log\big(m\big/|\widebar{\mathcal{I}}_0|\big)$ for some small constant $\epsilon>0$ yields
								%\begin{equation}\label{eq:hoeffding}
								%\mathbb{P}\!\left(\chi_{|\widebar{\mathcal{I}}_0|/2}>(1-\epsilon)\hat{\chi}_{|\widebar{\mathcal{I}}_0|/2} \right)\le {\rm e}^{-c_2\epsilon^2 (m/|\widebar{\mathcal{I}}_0|)^{2+2\epsilon}\log^2(m/|\widebar{\mathcal{I}}_0|)
								%}.
								%\end{equation}
								The remaining part in this section assumes that this event 
								occurs.
								
								% \asymp
								% \gtrsim
								% \lesssim
								
								Choosing $\xi:=4\log n$ and substituting this into the ccdf in \eqref{eq:chiccdf} leads to
								\begin{equation}\label{eq:chibound}
								\mathbb{P}\left(\chi\le 4\log n \right)= 
								1-1/n^2.
								\end{equation}
								Notice that each summand in $\sum_{i=1}^{|\widebar{\mathcal{I}}_0|/2}\chi_{[i]}\ge \sum_{i=1}^{m/2}\chi_i\mathbb{1}_{\tilde{\mathcal{E}}_i}$ is Chi-square distributed, and hence could be unbounded, so we choose to work with the truncation $\sum_{i=1}^{m/2}\chi_i\mathbb{1}_{\tilde{\mathcal{E}}_i}$, where the $\mathbb{1}_{\tilde{\mathcal{E}}_i}$'s are independent copies of $\mathbb{1}_{\tilde{\mathcal{E}}}$, and $\mathbb{1}_{\tilde{\mathcal{E}}}$
								denotes the indicator function for the ensuing events
								\begin{equation}\label{eq:event}
								\tilde{\mathcal{E}}:=\left\{\chi\ge \hat{\chi}_{|\widebar{\mathcal{I}}_0|/2}\right\}\cap\left\{\chi\le 4\log n \right\}.
								\end{equation}
								Apparently, it holds that $\sum_{i=1}^{|\widebar{\mathcal{I}}_0|/2}\chi_{[i]}\ge \sum_{i=1}^{m/2}\chi_i\mathbb{1}_{\tilde{\mathcal{E}}_i}$.
								One further establishes that 
								\begin{align}\label{eq:tmean}
								\mathbb{E}\left[\chi_i\mathbb{1}_{\tilde{\mathcal{E}}_i}\right]:\!&=\int_{\hat{\chi}_{|\widebar{\mathcal{I}}_0|/2}}^{4\log n} \frac{1}{2}r{\rm e}^{-r/2}{\rm d}r\nonumber\\
								&=\left( \hat{\chi}_{|\widebar{\mathcal{I}}_0|/2}\!+2\right){\rm e}^{-{\hat{\chi}_{|\widebar{\mathcal{I}}_0|/2}}/{2}} \!-\left(4\log n+2\right){\rm e}^{-2\log n}\nonumber\\
								&=\frac{2|\widebar{\mathcal{I}}_0|}{m}\left[1+\log \big(m\big/|\widebar{\mathcal{I}}_0\big)\right]-\frac{\left(4\log n + 2\right)}{n^2}.
								\end{align}
								
								The task of bounding $\sum_{i=1}^{|\widebar{\mathcal{I}}_0|}a_{[i],1}^2$ in~\eqref{eq:relation} 
								now boils down to bounding $\sum_{i=1}^{m/2}\chi_i\mathbb{1}_{\tilde{\mathcal{E}}_i}$ from its expectation in \eqref{eq:tmean}.    
								A convenient way to accomplish this is using the Bernstein inequality~\cite[Proposition 5.16]{chap2010vershynin}, that deals with bounded random variables. That also justifies introducing the upper-bound truncation on $\chi$ in \eqref{eq:event}. Specifically, define
								\begin{equation}
								\label{eq:zeta}
								\vartheta_i:=\chi_i\mathbb{1}_{\tilde{\mathcal{E}}_i}-\mathbb{E}\left[\chi_i\mathbb{1}_{\tilde{\mathcal{E}}_i}\right],\quad 1\le i\le m/2.
								\end{equation}
								Thus, $\left\{\vartheta_i\right\}_{i=1}^{m/2}$ are i.i.d. centered and bounded random variables following from the mean-subtraction and the upper-bound truncation. Further, according to the ccdf~\eqref{eq:chiccdf} and the definition of sub-exponential random variables~\cite[Definition 5.13]{chap2010vershynin}, the terms $\left\{\vartheta_i\right\}_{i=1}^{m/2}$ are sub-exponential. 
								Then, the following 
								\begin{equation}
								\label{eq:meanbound}
								\Big|\sum_{i=1}^{m/2}\vartheta_i\Big|\ge \tau
								\end{equation}
								holds with probability at least $1-2{\rm e}^{-c_s\min\left({\tau}/{K_s},{\tau^2}/{K_s^2}\right)}$, in which $c_s>0$ is a universal constant, and $K_s:=\max_{i\in [m/2]}\|\vartheta_i\|_{\psi_1}$ represents the maximum subexponential norm of the $\vartheta_i$'s. 
								
								Indeed, $K_s$ can be found as follows~\cite[Definition 5.13]{chap2010vershynin}:
								\begin{align}\label{eq:subnorm}
								K_s:\!&=\sup_{p\ge 1}p^{-1}\left(\mathbb{E}\left[|\vartheta_i|^p\right]\right)^{1/p}\nonumber\\
								&\le \left(4\log n-2\log\big(m\big/|\widebar{\mathcal{I}}_0|\big)\right) \left[|\widebar{\mathcal{I}}_0|\big/m-1/n^2\right]\nonumber\\
								&\le \frac{2|\widebar{\mathcal{I}}_0|}{m}\log\left(n^2|\widebar{\mathcal{I}}_0|\big/m\right)\nonumber\\
								&\le \frac{4|\widebar{\mathcal{I}}_0|}{m}\log n.
								\end{align}
								Choosing $\tau:=8|\widebar{\mathcal{I}}_0|/(c_sm)\cdot\log^2 n$ in \eqref{eq:meanbound} yields
								\begin{align}
								\label{eq:zetabound}
								\sum_{i=1}^{m/2}\chi_i\mathbb{1}_{\tilde{\mathcal{E}}_i}&\ge |\widebar{\mathcal{I}}_0|\left[1+\log \big(m\big/|\widebar{\mathcal{I}}_0|\big)\right]-8|\widebar{\mathcal{I}}_0|/(c_sm)\cdot\log^2 n
								\nonumber\\
								&\quad\, 
								-{m\left(2\log n + 1\right)}/{n^2}\nonumber\\
								&\ge (1-\epsilon_s)|\widebar{\mathcal{I}}_0|\left[1+\log \big(m\big/|\widebar{\mathcal{I}}_0|\big)\right]
								%\nonumber\\ &\ge \left(1-\epsilon_s\right)|\widebar{\mathcal{I}}_0|\left[1+\log \big(m\big/|\widebar{\mathcal{I}}_0|\big)\right]
								\end{align}
								for some small constant $\epsilon_s >0$, which 
								holds with probability at least $1-m{\rm e}^{-n/2}-{\rm e}^{-c_{0}m}-1/n^2$ as long as $m/n$ exceeds some numerical constant and $n$ is sufficiently large.
								Therefore, combining~\eqref{eq:down},~\eqref{eq:relation}, and~\eqref{eq:zetabound}, 
								one concludes that the following holds with high probability
								\begin{equation}\label{eq:low}
								\big\|\widebar{\bm{S}}_0\bm{x}\big\|^2=\sum_{i=1}^{|\widebar{\mathcal{I}}_0|}\frac{a_{i,1}^2}{\left\|\bm{a}_{i}\right\|^2}\ge (1-\epsilon_s)\frac{|\widebar{\mathcal{I}}_0|}{2.3n}\left[1+\log \big(m\big/|\widebar{\mathcal{I}}_0|\big)\right].
								\end{equation}
								%which is true with high probability.
								% at least $1-{\rm e}^{-c_{\rm x}m}-1/n^2-m{\rm e}^{-n/2}$. 
								Taking $\epsilon_s:=0.01$ without loss of generality concludes the proof of Lemma~\ref{lem:low}.  
								%and putting the upper
								%and lower bounds in~\eqref{eq:up} and~\eqref{eq:low}
								% together, one summarizes that
								%\begin{align}\label{eq:fbound}
								%%\sin^2\theta=
								%\frac{\big\|\widebar{\bm{S}}_0\bm{u}\big\|^2}{\big\|\widebar{\bm{S}}_0\bm{x}\big\|^2}\le \frac{2.4}{1+\log\big(m/|\widebar{\mathcal{I}}_0|\big)}:=\kappa
								%\end{align}
								%which holds with probability at least $1-(m+3){\rm e}^{-n/2}-{\rm e}^{-c_0m}-1/n^2$, with the proviso that $m\ge c_1' |\widebar{\mathcal{I}}_0|$, and $m\ge c_2' n$, $|\widebar{\mathcal{I}}_0|\ge c_3' n$ for some absolute constants $c_1',\,c_2',\,c_3'>0$, and sufficiently large $n$. 

								%%%%%%%%%%%%%%%%%%%%%%%%%%%%%%%%%%%%%%%%%%%%%%%%%%%%%%%%%%%%%%%%%%%%%%%%%%%
								
								\subsection{Proof of Lemma~\ref{le:1stterm}}\label{proof:1stterm}
								%Argue this first for a given pair of $\bm{z}$ and $\bm{x}$, so $\bm{h}=\bm{z}-\bm{x}$ is fixed as well. 
								%
								
								%Without loss of generality, assume $\|\bm{x}\|=1$. 
								Let us first prove the argument for a fixed pair $\bm{h}$ and $\bm{x}$, such that $\bm{h}$ and $\bm{z}$ are independent of $\{\bm{a}_i\}_{i=1}^m$, and then apply a covering argument. 
								To start, introduce a Lipschitz-continuous counterpart for the discontinuous indicator function~\cite[A.2]{twf}
								\begin{equation}
								\chi_E(\theta):=\left\{\begin{array}
								{lll}
								1,&|\theta|\ge \frac{\sqrt{1.01}}{1+\gamma},\\
								{100(1+\gamma)^2\theta^2-100},&\frac{1}{1+\gamma}\le 
								|\theta|<\frac{\sqrt{1.01}}{1+\gamma},\\
								0,&|\theta|<\frac{1}{1+\gamma}
								\end{array}\right.
								\end{equation}
								with Lipschitz constant $\mathcal{O}(1)$. 
								Recall that $\mathcal{E}_i=\left\{\left|\frac{\bm{a}_i^\ccalT\bm{z}}{\bm{a}_i^\ccalT\bm{x}}\right|\ge \frac{1}{1+\gamma}\right\}$, so it holds that $0\le \chi_E\left(\left|\frac{\bm{a}_i^\ccalT\bm{z}}{\bm{a}_i^\ccalT\bm{x}}\right|\right)\le \mathbb{1}_{\mathcal{E}_i}$ for any $\bm{x}\in\mathbb{R}^n$ and $\bm{h}\in\mathbb{R}^n$, thus yielding
								\begin{align}
								\frac{1}{m}\sum_{i=1}^m\left(\bm{a}_i^\ccalT\bm{h}\right)^2\mathbb{1}_{\mathcal{E}_i}&\ge \frac{1}{m}\sum_{i=1}^m\left(\bm{a}_i^\ccalT\bm{h}\right)^2\chi_E\left(\left|\frac{\bm{a}_i^\ccalT\bm{z}}{\bm{a}_i^\ccalT\bm{x}}\right|\right)
								\nonumber\\
								&	=\frac{1}{m}\sum_{i=1}^m\left(\bm{a}_i^\ccalT\bm{h}\right)^2\chi_E\left(\left|1+\frac{\bm{a}_i^\ccalT\bm{h}}{\bm{a}_i^\ccalT\bm{x}}\right|\right)
								.\label{eq:1term2}
								\end{align}
								
								By homogeneity and rotational invariance of normal distributions, it suffices to prove the case where $\bm{x}=\bm{e}_1$ and $\|\bm{h}\|/\|\bm{x}\|=\|\bm{h}\|\le \rho$. 
								%Argue this first for a given vector $\bm{z}$ such that ${\|\bm{h}\|}/{\|\bm{x}\|}=\|\bm{h}\|\le \rho$. 
								According to~\eqref{eq:1term2}, lower bounding the first term in~\eqref{eq:target} can be achieved by lower bounding $\sum_{i=1}^m(\bm{a}_i^\ccalT\bm{h})^2\chi_E\left( \left|1+\frac{\bm{a}_i^\ccalT\bm{h}}{\bm{a}_i^\ccalT\bm{x}}\right|\right)$ instead. To that end, let us find the mean of $\left(\bm{a}_i^\ccalT\bm{h}\right)^2\chi_E\left( \left|1+\frac{\bm{a}_i^\ccalT\bm{h}}{\bm{a}_i^\ccalT\bm{x}}\right|\right)$. Note that $\left(\bm{a}_i^\ccalT\bm{h}\right)^2$ and $\chi_E\left( \left|1+\frac{\bm{a}_i^\ccalT\bm{h}}{\bm{a}_i^\ccalT\bm{x}}\right|\right)$ are dependent. Introduce an orthonormal matrix $\bm{U}_{\bm{h}}$ that contains $\bm{h}^\ccalT/\|\bm{h}\|$ as its first row, i.e.,
								\begin{equation}
								\bm{U}_{\bm{h}}:=\left[\begin{array}
								{c}
								\bm{h}^\ccalT/\|\bm{h}\|\\
								\widetilde{\bm{U}}_{\bm{h}}
								\end{array}
								\right]
								\end{equation} 
								for some orthogonal matrix $\widetilde{\bm{U}}_{\bm{h}}\in\mathbb{R}^{(n-1)\times n}$ such that $\bm{U}_{\bm{h}}$ is orthonormal. Moreover, define $\tilde{\bm{h}}:=\bm{U}_{\bm{h}}\bm{h}$, and $\tilde{\bm{a}}_i:=\bm{U}_{\bm{h}}\bm{a}_i$; and let $\tilde{a}_{i,1}$ and $\tilde{\bm{a}}_{i,\backslash 1}$ denote the first entry and the remaining entries in the vector $\tilde{\bm{a}}_i$; likewise for $\tilde{\bm{h}}$. Then, for any $\bm{h}$ such that $\|\bm{h}\|\le \rho$, we have
								\begin{align}
								&\mathbb{E}\left[(\bm{a}_i^\ccalT\bm{h})^2\chi_E\left( \left|1+\frac{\bm{a}_i^\ccalT\bm{h}}{\bm{a}_i^\ccalT\bm{x}}\right|\right)\right]\nonumber\\
								&=\mathbb{E}\left[(\tilde{a}_{i,1}\tilde{h}_1)^2\chi_E\!\left(\left|1\!+\!
								\frac{\bm{a}_{i}^\ccalT\bm{h}}{\bm{a}_i^\ccalT\bm{x}}\right|\right)\right]\!+\!\mathbb{E}\left[(\tilde{\bm{a}}_{i,\backslash 1}^\ccalT\tilde{\bm{h}}_{\backslash 1})^2\chi_E\!\left(\left|1\!+\!\frac{\bm{a}_i^\ccalT\bm{h}}{\bm{a}_i^\ccalT\bm{x}}\right|\right)\right]\nonumber\\
								&=\tilde{h}_1^2\,\mathbb{E}\left[\tilde{a}_{i,1}^2\,\chi_E\left( \left|1+\frac{\bm{a}_i^\ccalT\bm{h}}{a_{i,1}}\right|\right)\right]
								+\mathbb{E}\left[(\tilde{\bm{a}}_{i,\backslash 1}^\ccalT\tilde{\bm{h}}_{\backslash 1})^2\right]\mathbb{E}\!\left[\chi_E\left( \left|1+
								\frac{\bm{a}_i^\ccalT\bm{h}}{a_{i,1}}
								\right|\right)\right]
								\nonumber\\
								&=\tilde{h}_1^2\mathbb{E}\!\left[\tilde{a}_{i,1}^2\chi_E\!\left( \left|1+\frac{\bm{a}_i^\ccalT\bm{h}}{a_{i,1}}\right|\right)\right]+\big\|\tilde{\bm{h}}_{\backslash 1}\big\|^2
								\mathbb{E}\!\left[\chi_E\!\left( \left|1\!+\!\frac{\bm{a}_i^\ccalT\bm{h}}{a_{i,1}}\right|\right)\right]\nonumber\\
								&\ge \left(\tilde{h}_1^2\!+\!\|\tilde{\bm{h}}_{\backslash 1}\|^2\right)\min\left\{\mathbb{E}\left[{a}_{i,1}^2\chi_E\left( \left|1+h_1+
								\frac{\bm{a}_{i,\backslash 1}^\ccalT\bm{h}_{\backslash 1}}{a_{i,1}}\right|\right)\right],\right.\nonumber\\
								&\hspace{1.6em} \left.\mathbb{E}\left[\chi_E\left(\left|1+h_1+\frac{\bm{a}_{i,\backslash 1}^\ccalT\bm{h}_{\backslash 1}}{a_{i,1}}\right|\right)\right]
								\right\}\nonumber\\
								&\ge \|\bm{h}\|^2\min\bigg\{\mathbb{E}\left[a_{i,1}^2\chi_E\left(\left|1-\rho+\frac{a_{i,2}}{a_{i,1}}\rho\right|
								\right)
								\right],\,\mathbb{E}\left[\chi_E\left(1-\rho+\frac{a_{i,2}}{a_{i,1}}\rho
								\bigg)
								\right]
								\right\}
								\nonumber\\
								&= (1-\zeta_1)\|\bm{h}\|^2\label{eq:1bound}
								\end{align}
								where the second equality follows from the independence between $\tilde{\bm{a}}_{i,\backslash 1}^\ccalT\tilde{\bm{h}}_{\backslash 1}$ and $\bm{a}_i^\ccalT\bm{h}$, the second inequality holds for $\rho\le 1/10$ and $\gamma\ge 1/2$, 
								and the last equality comes from the definition of $\zeta_1 $ in~\eqref{eq:zeta}. Notice that $\varrho:=(\bm{a}_i^\ccalT\bm{h})^2\chi_E\left( \left|1+\frac{\bm{a}_i^\ccalT\bm{h}}{\bm{a_i}^\ccalT\bm{x}}\right|\right)\le (\bm{a}_i^\ccalT\bm{h})^2\eqdef \|\bm{h}\|^2a_{i,1}^2$ is a subexponential variable, and thus its subexponential norm $\|\varrho\|_{\psi_1}:=\sup_{p\ge 1}\left[\mathbb{E}(|\varrho|^p)\right]^{1/p}$ is finite. %(Although it is possible to compute an upper bound on this subexponential norm, this is not pursued at the moment.) 
								
								Direct application of the Berstein-type inequality~\cite[Proposition 5.16]{chap2010vershynin} confirms that for any $\epsilon>0$, the following
								\begin{align}
								& \frac{1}{m}\sum_{i=1}^m\left(\bm{a}_i^\ccalT\bm{h}\right)^2\chi_E\left(\left|1+\frac{\bm{a}_i^\ccalT\bm{h}}{\bm{a}_i^\ccalT\bm{x}}\right|\right)\nonumber\\
								&\ge \mathbb{E}\left[\left(\bm{a}_i^\ccalT\bm{h}\right)^2\chi_E\left(\left|1+\frac{\bm{a}_i^\ccalT\bm{h}}{\bm{a}_i^\ccalT\bm{x}}\right|\right)\right]-\epsilon\|\bm{h}\|^2
								\nonumber\\
								&\ge   \left(1-\zeta_1-\epsilon\right)\|\bm{h}\|^2 	\label{eq:1sttermbound}
								\end{align} 
								holds with probability at least $1-{\rm e}^{-c_5m\epsilon^2}$ for some numerical constant $c_5>0$ provided that $\epsilon\le \|\varrho\|_{\psi_1}$ by assumption. 
								
								%We have proved the argument for a fixed $\|\bm{h}\|\le \rho$. 
								To obtain uniform control over all vectors $\bm{z}$ and $\bm{x}$ such that $\|\bm{z}-\bm{x}\|\le \rho$, 
								%To complete the argument,
								the net covering argument is applied~\cite[Definition 5.1]{chap2010vershynin}. 
								Let $\mathcal{S}_\epsilon$ be an $\epsilon$-net of the unit sphere, $\mathcal{L}_\epsilon$ be an $\epsilon$-net of $[0,\,\rho]$, and define
								\begin{equation}
								\mathcal{N}_{\epsilon}:=\left\{\left(\bm{z},\,\bm{h},\,t\right):\left(\bm{z}_0,\,\bm{h}_0,\,t_0\right)\in\mathcal{S}_\epsilon\times\mathcal{S}_\epsilon\times\mathcal{L}_\epsilon
								\right\}.
								\end{equation} 
								Since the cardinality $\left|\mathcal{S}_\epsilon\right|\le \left(1+2/\epsilon\right)^{n}$~\cite[Lemma 5.2]{chap2010vershynin}, then
								\begin{equation}
								\left|\mathcal{N}_\epsilon\right|\le \left(
								1+2/\epsilon\right)^{2n}\rho/\epsilon\le \left(1+2/\epsilon\right)^{2n+1}
								\end{equation}
								due to the fact that $\rho/\epsilon< 2/\epsilon< 1+2/\epsilon$ for $0< \rho< 1$.
								
								Consider now any $\left(\bm{z},\,\bm{h},\,t\right)$ obeying $\|\bm{h}\|=t\le \rho$. There exists a pair $\left(\bm{z}_0,\,\bm{h}_0,\,t_0\right)\in\mathcal{N}_\epsilon$ such that $\left\|\bm{z}-\bm{z}_0
								\right\|$, $\|\bm{h}-\bm{h}_0\|$, and $|t-t_0|$ are each at most $\epsilon$. Taking the union bound yields
								\begin{align}
								& \frac{1}{m}\sum_{i=1}^m\left(\bm{a}_i^\ccalT\bm{h}_0\right)^2\chi_E\left(\left|1+\frac{\bm{a}_i^\ccalT\bm{h}_0}{\bm{a}_i^\ccalT\bm{x}}\right|\right)\nonumber\\
								&\ge  \frac{1}{m}\sum_{i=1}^m\left(\bm{a}_i^\ccalT\bm{h}_0\right)^2\chi_E\left(\left|1-t_0+\frac{{a}_{i,2}}{{a}_{i,1}}t_0\right|\right)\nonumber\\
								%&\ge  \frac{1}{m}\sum_{i=1}^m\left(\bm{a}_i^\ccalT\bm{h}_0\right)^2\chi_E\left(\left|1-\rho+\frac{{a}_{i,2}}{{a}_{i,1}}\rho\right|\right)\nonumber\\
								& \ge   \left(1-\zeta_1-\epsilon \right)\|\bm{h}_0\|^2,\quad \forall \left(\bm{z}_0,\,\bm{h}_0,\,t_0\right)\in\mathcal{N}_\epsilon
								\end{align} 
								with probability at least $1-\left(1+2/\epsilon\right)^{2n+1}{\rm e}^{-c_5 \epsilon^2m}\ge 1-{\rm e}^{-c_0m}$, which follows by choosing $m$ such that $m\ge \left(c_6\cdot\epsilon^{-2}\log\epsilon^{-1}\right) n$ for some constant $c_6>0$.

								Recall that $\chi_E\left(\tau\right)$ is Lipschitz continuous, thus %$\forall \bm{h}$
								\begin{align}
								&\bigg|
								\frac{1}{m}\sum_{i=1}^m
								\left(\bm{a}_i^\ccalT\bm{h}\right)^2\chi_E\left(\left|1+\frac{\bm{a}_i^\ccalT\bm{h}}{\bm{a}_i^\ccalT\bm{x}}\right|\right)-
								\left(\bm{a}_i^\ccalT\bm{h}_0\right)^2\chi_E\left(\left|1+\frac{\bm{a}^\ccalT\bm{h}_0}{\bm{a}_i^\ccalT\bm{x}}\right|\right)
								\bigg|
								\nonumber\\
								&\lesssim \frac{1}{m}\sum_{i=1}^m\left|\left(\bm{a}_i^\ccalT\bm{h}\right)^2-\left(\bm{a}_i^\ccalT\bm{h}_0\right)^2
								\right|
								\nonumber\\
								&= \frac{1}{m}\sum_{i=1}^m\left|\bm{a}_i^\ccalT\left(\bm{h}\bm{h}^\ccalT-\bm{h}_0\bm{h}_0^\ccalT\right)\bm{a}_i
								\right|\nonumber\\
								&\lesssim c_7\sum_{i=1}^m\left|\bm{h}\bm{h}^\ccalT-\bm{h}_0\bm{h}_0^\ccalT
								\right|\nonumber\\
								&\le 2.5 c_{7}\left\|\bm{h}-\bm{h}_0\right\|\left\|\bm{h}\right\|\nonumber\\
								&\le 2.5c_7\rho \epsilon
								\end{align}
								for some numerical constant $c_7$ and provided that $\epsilon<1/2$ and  $m\ge \left(c_6\cdot\epsilon^{-2}\log\epsilon^{-1}\right) n$,  
								where the first inequality arises from the Lipschitz property of $\chi_E(\tau)$, the second uses the results in Lemma 1 in \cite{twf}, and the third from Lemma 2 in \cite{twf}.

								Putting all results together confirms that with probability exceeding $1-2{\rm e}^{-c_0m}$, we have
								\begin{align}
								&\frac{1}{m}\sum_{i=1}^m\left(\bm{a}_i^\ccalT\bm{h}\right)^2\chi_E\left(\left|1+\frac{\bm{a}_i^\ccalT\bm{h}}{\bm{a}_i^\ccalT\bm{x}}\right|\right)\nonumber\\
								&\quad \,
								\ge   \left[1-\zeta_1-\left(1+2.5c_7\rho\right)\epsilon\right]\left\|\bm{h}\right\|^2
								\end{align} 
								for all vectors $\left\|\bm{h}\right\|/\left\|\bm{x}\right\|\le\rho $, concluding the proof.

								\subsection{Proof of Lemma~\ref{le:2ndterm}}\label{sec:rare}
								Similar to the proof in Section~\ref{proof:1stterm}, it is convenient to work with the following auxiliary function instead of the discontinuous indicator function
								\begin{equation}
								\chi_D(\theta)\!:=\!\left\{\!\!\begin{array}
								{ll}
								1,&|\theta|\ge\frac{2+\gamma}{1+\gamma}\\
								{-100\left(\frac{1+\gamma}{2+\gamma}\right)^2\theta^2+100},&\sqrt{0.99}\cdot\frac{2+\gamma}{1+\gamma}\le\! 
								|\theta|<\!\frac{2+\gamma}{1+\gamma}\\
								0,&|\theta|<\sqrt{0.99}\cdot\frac{2+\gamma}{1+\gamma}
								\end{array}\right.
								\end{equation}
								which is Lipschitz continuous in $\theta$ with Lipschitz constant $\mathcal{O}(1)$.  
								For $\mathcal{D}_i=\left\{\left|\frac{\bm{a}_i^\ccalT\bm{h}}{\bm{a}_i^\ccalT\bm{x}}\right|\ge \frac{2+\gamma}{1+\gamma}\right\}$, it holds that $0\le \mathbb{1}_{\mathcal{D}_i}\le \chi_D\left(\left|\frac{\bm{a}_i^\ccalT\bm{h}}{\bm{a}_i^\ccalT\bm{x}}\right|\right)$ for any $\bm{x}\in\mathbb{R}^n$ and $\bm{h}\in\mathbb{R}^n$.
								%, thus leading to
								%\begin{equation}
								%	\frac{1}{m}\sum_{i=1}^m\mathbb{1}_{\mathcal{D}_i}
								%	\le \frac{1}{m}\sum_{i=1}^m\chi_D\left(\left|\frac{\bm{a}_i^\ccalT\bm{z}}{\bm{a}_i^\ccalT\bm{x}}\right|\right)
								%	=\frac{1}{m}\sum_{i=1}^m\chi_D\left(\left|1+\frac{\bm{a}_i^\ccalT\bm{h}}{\bm{a}_i^\ccalT\bm{x}}\right|\right)
								%	.\label{eq:2term2}
								%\end{equation}
								Assume without loss of generality that $\bm{x}=\bm{e}_1$.  Then for $\gamma> 0$ and $\rho\le 1/10$, it holds that
								\begin{align}
								\frac{1}{m}&\sum_{i=1}^m\mathbb{1}_{\Big\{\frac{|\bm{a}_i^\ccalT\bm{h}|}{
										|\bm{a}_i^\ccalT\bm{x}|}\ge \frac{2+\gamma}{1+\gamma}\Big\}}
										\le \frac{1}{m}\sum_{i=1}^m\chi_D\left(\left|\frac{\bm{a}_i^\ccalT\bm{h}}{\bm{a}_i^\ccalT\bm{x}}\right|\right)	%=\frac{1}{m}\sum_{i=1}^m\chi_D\left(\left|1+\frac{\bm{a}_i^\ccalT\bm{h}}{\bm{a}_i^\ccalT\bm{x}}\right\right)\nonumber %\allowdisplaybreaks
										\nonumber\\
										&	
										=\frac{1}{m}\sum_{i=1}^m\chi_D\left(\left|\frac{\bm{a}_i^\ccalT\bm{h}}{a_{i,1}}\right|\right)\nonumber\\ 
										&=\frac{1}{m}\sum_{i=1}^m\chi_D\left(\left|h_1+\frac{\bm{a}_{i,\backslash 1}^\ccalT\bm{h}_{\backslash 1}}{a_{i,1}}\right|\right)\nonumber\\
										&=\frac{1}{m}\sum_{i=1}^m\chi_D\left(\left|h_1+\frac{a_{i,2}}{a_{i,1}}\left\|\bm{h}_{\backslash 1}\right\|\right|\right)\nonumber\\
										&\overset{\rm (i)}{\le}\frac{1}{m}\sum_{i=1}^m\mathbb{1}_{\left\{
											\left|h_1+\frac{a_{i,2}}{a_{i,1}}\|\bm{h}_{\backslash 1}\|\right|\ge \sqrt{0.99}\cdot\frac{2+\gamma}{1+\gamma}
											\right\}}
											\end{align}
											where the last inequality arises from the definition of $\chi_D$. 
											Note that $a_{i,2}/a_{i,1}$ obeys the standard Cauchy distribution, i.e., $a_{i,2}/a_{i,1}\sim{\rm Cauchy(0,1)}$ \cite{1962cauchy}. Transformation properties of Cauchy distributions assert that $h_1+\frac{a_{i,2}}{a_{i,1}}\|\bm{h}_{\backslash 1}\|\sim{\rm Cauchy}(h_1,\|\bm{h}_{\backslash 1}\|)$~\cite{2014cauchy}. Recall that the cdf of a Cauchy distributed random variable $w\sim{\rm Cauchy}\left(\mu_0,\alpha\right)$ is given by~\cite{1962cauchy} 
											\begin{equation}
											F(w;\mu_0,\alpha)=\frac{1}{\pi}\arctan\left(\frac{w-\mu_0}{\alpha}\right)+\frac{1}{2}.
											\end{equation}
											It is easy to check that when $\|\bm{h}_{\backslash 1}\|=0$, the indicator function $\mathbb{1}_{\mathcal{D}_i}=0$ due to $|h_1|\le \rho< \sqrt{0.99}(2+\gamma)/(1+\gamma)$. Consider only $\|\bm{h}_{\backslash 1}\|\ne 0$ next. 
											Define for notational brevity $w:=a_{i,2}/a_{i,1}$, $\alpha:=\|\bm{h}_{\backslash 1}\|$, as well as $\mu_0:=h_1/\alpha$ and $w_0:=\sqrt{0.99}\frac{2+\gamma}{\alpha(1+\gamma)}$. Then, 
											\begin{align}
											\mathbb{E}&[\mathbb{1}_{
												\{
												|\mu_0+w|\ge w_0
												\}}]
												=1-\big[F
												(w_0;\mu_0,1)-F
												(-w_0;\mu_0,1)\big]\nonumber\\
												&=1-\frac{1}{\pi}\big[\arctan({w_0-\mu_0})-\arctan({-w_0-\mu_0})\big]
												\nonumber\\
												&\overset{\rm (i)}{=}\frac{1}{\pi}\arctan\!\left(\frac{2w_0}{w_0^2-\mu_0^2-1}\right)
												\nonumber\\
												&\overset{\rm (ii)}{\le}
												\frac{1}{\pi}\cdot\frac{2w_0}{w_0^2-\mu_0^2-1}
												\nonumber\\
												%&\le \frac{2}{\pi}\cdot\frac{\sqrt{0.99}}{0.99(2+\gamma)/(1+\gamma)-(1+2\rho^2)(1+\gamma)/(2+\gamma)}\rho\nonumber\\
												%&\le\frac{2}{\pi}\cdot\frac{\sqrt{0.99}}{0.99(2+\gamma)/(1+\gamma)-1}\rho\nonumber\\
												%&\le\frac{2}{\pi}\cdot\frac{\sqrt{0.99}(1+\gamma)}{0.98-0.01\gamma}\rho\nonumber\\
												&\overset{\rm (iii)}{\le}\frac{1}{\pi}\cdot\frac{2\sqrt{0.99}\rho(2+\gamma)/(1+\gamma)}{0.99(2+\gamma)^2/(1+\gamma)^2-\rho^2}\nonumber\\
												%&\overset{\rm (iii)}{\le}\frac{1}{\pi}\cdot\frac{2\sqrt{0.99}\|\bm{h}_{\backslash 1}\|(2+\gamma)/(1+\gamma)}{0.99(2+\gamma)^2/(1+\gamma)^2-\|\bm{h}\|^2}\nonumber\\
												%&\le \frac{2\sqrt{0.99}\rho}{\pi(0.99-\rho^2)}\nonumber\\
												&\le 0.0646
												\label{eq:prob11}
												%\nonumber\\ &\overset{\rm (ii)}{\le} 0.482
												\end{align}
												for all $\gamma> 0$ and $\rho\le 1/10$.
												%	provided that $\gamma$ and $\rho$ are chosen such that $0.99(2+\gamma)^2/(1+\gamma)^2> (1+2\rho+2\rho^2)$, which holds true for $1/2\le \gamma\le 4$ and $\rho \le 1/10$. 
												In deriving $\rm (i)$, we used the property $\arctan(u)+\arctan(v)=\arctan\!\left(\frac{u+v}{1-uv}\right) ~({\rm mod}~\pi)$ for any $uv\ne 1$. Concerning $\rm (ii)$, the inequality $\arctan(x)\le x$ for $x\ge 0$ is employed. Plugging given parameter values and using $\|\bm{h}_{\backslash 1}\|\le \|\bm{h}\|\le \rho$  confirms ${\rm (iii)}$. 
												%The bound in $(\rm ii)$ is rather loose, yet it suffices for our purpose. Note that $\frac{\sqrt{0.99}(1+\gamma)}{0.42\pi}$ is $\mathcal{O}(1)$, so the probability in~\eqref{eq:prob11} is on the order of $\rho$, which can be made arbitrarily small as demonstrated by our analysis in Section~\ref{subsec:initial}.   
												%	Specifically, when taking values $\gamma=0.7$ and $\rho=1/10$, it holds $ \mathbb{1}_{
												%	\left\{
												%	\left|\mu_0+z\right|\ge z_0
												%	\right\}}\le 0.13$. 
												Next, $\mathbb{1}_{
													\left\{
													\left|\mu_0+w\right|\ge w_0
													\right\}}$ is bounded; and it is known that all bounded random variables are subexponential. Thus, upon applying the Bernstein-type inequality~\cite[Corollary 5.17]{chap2010vershynin},   
													the next holds with probability at least $1-{\rm e}^{-c_5m\epsilon^2}$ for some numerical constant $c_5>0$ and any sufficiently small $\epsilon> 0$:
													\begin{align}
													\frac{1}{m}\sum_{i=1}^m\mathbb{1}_{\left\{\frac{\left|\bm{a}_i^\ccalT\bm{h}\right|}{
															\left|\bm{a}_i^\ccalT\bm{x}\right|}\ge \frac{2+\gamma}{1+\gamma}\right\}}
															&\le \frac{1}{m}\sum_{i=1}^m\mathbb{1}_{
																\left\{
																\left|h_1+\frac{a_{i,2}}{a_{i,1}}\|\bm{h}_{\backslash 1}\|\right|\ge \sqrt{0.99}\frac{2+\gamma}{1+\gamma}
																\right\}
																}\nonumber\\
																&
																\le (1+\epsilon)\mathbb{E}\Big[\mathbb{1}_{
																	\left\{
																	\left|h_1+\frac{a_{i,2}}{a_{i,1}}\|\bm{h}_{\backslash 1}\|\right|\ge \sqrt{0.99}\frac{2+\gamma}{1+\gamma}
																	\right\}
																	}\Big]\nonumber\\
																	&\le\frac{1+\epsilon}{\pi}\cdot\frac{2\sqrt{0.99}\rho(2+\gamma)/(1+\gamma)}{0.99(2+\gamma)^2/(1+\gamma)^2-\rho^2}.\label{eq:inter1}
																	\end{align}
																	
																	On the other hand, it is easy to establish that the following holds true for any fixed 
																	$ \bm{h}\in\mathbb{R}^n$:
																	\begin{align}
																	\mathbb{E}\left[(\bm{a}_i^\ccalT\bm{h})^4\right]=\mathbb{E}\left[a_{i,1}^4\right]\left\|\bm{h}\right\|^4=3\left\|\bm{h}\right\|^4
																	\end{align}
																	which has also been used in Lemma 1~\cite{twf} and Lemma 6.1~\cite{sun2016}. 
																	Furthermore, recalling our working assumption $\|\bm{a}_i\|\le \sqrt{2.3n}$ and $\|\bm{h}\|\le \rho \|\bm{x}\|$, the random variables $(\bm{a}_i^\ccalT\bm{h})^4$ are bounded, and thus they are subexponential~\cite{chap2010vershynin}.  Appealing again to the Bernstein-type inequality for subexponential random variables \cite[Proposition 5.16]{chap2010vershynin} and provided that $m/n>c_6\cdot \epsilon^{-2}\log\epsilon^{-1}$ for some numerical constant $c_6>0$, we have 
																	\begin{align}
																	\frac{1}{m}\sum_{i=1}^m\left(\bm{a}_i^\ccalT\bm{h}\right)^4\le 3(1+\epsilon)\left\|\bm{h}\right\|^4\label{eq:inter2}
																	\end{align}
																	which holds with probability exceeding $1-{\rm e}^{-c_5m\epsilon^2}$ for some universal constant $c_5>0$ and  any sufficiently small $\epsilon> 0$. 
																	
																	Combining results \eqref{eq:inter1}, \eqref{eq:inter2}, leveraging the Cauchy-Schwartz inequality, and considering $\mathcal{D}_i\cap\mathcal{K}_i$ only consisting of a spherical cap, the following holds for any $ \rho\le 1/10$ and $  \gamma> 0$:
																	\begin{align}
																	&	\frac{1}{m}\sum_{i=1}^m
																	\left(\bm{a}_i^\ccalT\bm{h}\right)^2\mathbb{1}_{\mathcal{D}_i\cap \mathcal{K}_i}\nonumber\\
																	&\le \sqrt{\frac{1}{m}\sum_{i=1}^m\left(\bm{a}_i^\ccalT\bm{h}\right)^4}
																	\sqrt{\frac{1}{2}\cdot\frac{1}{m}\sum_{i=1}^m\mathbb{1}_{\left\{\frac{\left|\bm{a}_i^\ccalT\bm{h}\right|}{
																				\left|\bm{a}_i^\ccalT\bm{x}\right|}\ge \frac{2+\gamma}{1+\gamma}\right\}}}\nonumber\\
																				&\le \sqrt{3(1+\epsilon)\left\|\bm{h}\right\|^4}\sqrt{\frac{1+\epsilon}{\pi}\cdot\frac{\sqrt{0.99}\rho(2+\gamma)/(1+\gamma)}{0.99(2+\gamma)^2/(1+\gamma)^2-\rho^2}
																					}\nonumber\\
																					%&=1.5(1+\epsilon)\sqrt{1+\gamma}\sqrt{\rho}\left\|\bm{h}\right\|^2\nonumber\\
																					& \overset{\Delta}{=} (\zeta_2'+\epsilon')\left\|\bm{h}\right\|^2
																					\end{align}
																					where $\zeta_2':=0.9748\sqrt{\rho\tau/(0.99\tau^2-\rho^2)}$ with $\tau:=(2+\gamma)/(1+\gamma)$, which
																					holds with probability at least $1-2{\rm e}^{-c_0m}$. The latter arises upon choosing $c_0\le c_5\epsilon^2$ in 
																					$1-2{\rm e}^{-c_5m\epsilon^2}$, which can be accomplished by taking $m/n$ sufficiently large.
